# Supplementary material for: Diffusion Imitation from Observation
Source: arXiv:2410.05429 source file (2024-10-07)
Supplement: Supplementary file 1 [file converge_performance.tex]

\section{Converged Performance}
\label{appendix:converge}

\begin{table*}

\centering
% \scriptsize
\caption[Converged Performance]{\textbf{Converged Performance.} 
We report the quantitative results of the converged performance across all experiments.
}%\ra{1.3}
\scalebox{0.6}{\begin{tabular}{cc|cccccc}
\toprule
Environments & Settings & BC & Diffusion Policy & GAIL & WAIL & BCO & \method{} \\
\midrule
& & \multicolumn{5}{c}{\textbf{Main Results}} \\
\midrule
\fetchpush{} &  & $82.00\%\pm21.13\%$ & $89.40\%\pm2.06\%$ & $33.73\%\pm37.63\%$ & $91.64\%\pm9.08\%$ & \hl{$93.66\%\pm3.15\%$} & \hl{$95.78\%\pm0.80\%$} \\
\walker {} &  & \hl{$5431.19\pm267.40$} & $4749.03\pm224.96$ & $3581.18\pm574.20$ & $2521.07\pm863.44$ & $4639.47\pm282.92$ & \hl{$5381.15\pm115.25$}\\
\carracing &  & $534.92\pm45.02$ & $592.20\pm103.17$ & $297.63\pm294.52$ & $-72.39\pm30.54$ & $689.62\pm96.72$ & \hl{$746.35\pm31.28$}\\
\midrule
& & \multicolumn{5}{c}{\textbf{Generalization Experiments}} \\
\midrule
\multirow{4}{*}{\fetchpush{}} 
 & 25\% & $52.67\%\pm6.18\%$ & $52.00\%\pm0.82\%$ & $33.05\%\pm9.35\%$ & $32.53\%\pm6.33\%$ & \hl{$89.67\%\pm4.33\%$} & \hl{$91.00\%\pm3.24\%$} \\
 & 50\% & $61.60\%\pm3.98\%$ & $68.80\%\pm1.72\%$ & $68.62\%\pm8.35\%$ & $63.85\%\pm5.77\%$ & $94.06\%\pm1.67\%$ & \hl{$96.83\%\pm0.49\%$} \\
 & 75\%  & $87.00\%\pm0.00\%$ & $86.00\%\pm2.45\%$ & $88.87\%\pm5.79\%$ & $72.47\%\pm1.05\%$ & \hl{$96.58\%\pm0.31\%$} & \hl{$96.83\%\pm0.58\%$} \\
 & 100\% & $91.00\%\pm0.82\%$ & $93.03\%\pm2.13\%$ & $95.47\%\pm0.35\%$ & $69.52\%\pm2.60\%$ & \hl{$98.43\%\pm0.12\%$} & \hl{$98.20\%\pm0.04\%$} \\
 \cmidrule{2-8}
 \multirow{5}{*}{\fetchpush{}} 
 & $1.00 \times$  & $47.40\%\pm31.10\%$ & $92.40\%\pm2.58\%$ & $18.37\%\pm36.74\%$ & $0.00\%\pm0.00\%$ & $49.24\%\pm42.53\%$ & \hl{$97.79\%\pm1.27\%$} \\
 & $1.25 \times$  & $44.00\%\pm30.63\%$ & \hl{$85.40\%\pm8.40\%$} & $8.57\%\pm16.92\%$ & $0.00\%\pm0.00\%$ & $37.03\%\pm45.36\%$ & \hl{$89.22\%\pm2.20\%$} \\
 & $1.50 \times$  & $40.60\%\pm27.62\%$ & \hl{$80.00\%\pm7.13\%$} & $19.03\%\pm38.06\%$ & $0.00\%\pm0.00\%$ & $33.97\%\pm41.61\%$ & \hl{$86.90\%\pm1.90\%$} \\
 & $1.75 \times$  & $33.80\%\pm23.96\%$ & \hl{$76.06\%\pm7.48\%$} & $19.15\%\pm38.25\%$ & $0.00\%\pm0.00\%$ & $2.14\%\pm4.28\%$ & $49.86\%\pm40.73\%$ \\
 & $2.00 \times$  & $28.80\%\pm22.68\%$ & $76.64\%\pm7.63\%$ & $39.17\%\pm47.98\%$ & $0.00\%\pm0.00\%$ & $0.00\%\pm0.00\%$ & \hl{$87.22\%\pm1.93\%$} \\
 \cmidrule{2-8}
 \multirow{5}{*}{\fetchpush{}} 
 & $1.00 \times$  & $96.00\%\pm6.10\%$ & $98.60\%\pm0.49\%$ & $94.18\%\pm4.87\%$ & \hl{$99.68\%\pm0.30\%$} & $98.12\%\pm0.75\%$ & $97.90\%\pm0.53\%$ \\
 & $1.25 \times$  & $88.80\%\pm17.07\%$ & \hl{$97.20\%\pm0.98\%$} & $94.34\%\pm1.62\%$ & $79.32\%\pm39.66\%$ & $75.66\%\pm37.86\%$ & \hl{$95.84\%\pm1.18\%$} \\
 & $1.50 \times$    & $82.00\%\pm21.13\%$ & $89.40\%\pm2.06\%$ & $33.73\%\pm37.63\%$ & $91.64\%\pm9.08\%$ & $93.66\%\pm3.15\%$ & $95.78\%\pm0.80\%$ \\
 & $1.75 \times$   & $71.00\%\pm23.13\%$ & $84.80\%\pm2.32\%$ & $43.71\%\pm36.51\%$ & $0.00\%\pm0.00\%$ & $55.62\%\pm45.56\%$ & \hl{$96.15\%\pm2.33\%$} \\
 & $2.00 \times$   & $64.40\%\pm21.70\%$ & $79.20\%\pm3.76\%$ & $16.89\%\pm25.08\%$ & $0.00\%\pm0.00\%$ & $40.90\%\pm47.59\%$ & \hl{$99.09\%\pm0.47\%$} \\
 \cmidrule{2-8}
 \multirow{5}{*}{\walker{}} 
 & $1.00 \times$   & $94.03\%\pm2.90\%$ & $95.06\%\pm2.16\%$ & $72.78\%\pm33.57\%$ & $51.95\%\pm36.88\%$ & \hl{$98.60\%\pm0.16\%$} & \hl{$98.32\%\pm0.39\%$} \\
 & $1.25 \times$  & $93.00\%\pm2.94\%$ & $92.71\%\pm1.27\%$ & $62.05\%\pm41.21\%$ & $28.30\%\pm38.68\%$ & \hl{$98.03\%\pm0.61\%$} & \hl{$97.17\%\pm1.50\%$ }\\
 & $1.50 \times$   & $91.31\%\pm2.61\%$ & $93.24\%\pm1.61\%$ & $43.82\%\pm35.31\%$ & $29.39\%\pm35.65\%$ & \hl{$97.49\%\pm0.48\%$} & $93.88\%\pm3.23\%$ \\
 & $1.75 \times$   & $89.67\%\pm1.70\%$ & $92.00\%\pm0.82\%$ & $60.32\%\pm27.33\%$ & $28.12\%\pm37.87\%$ & \hl{$96.20\%\pm0.25\%$} & $91.73\%\pm3.18\%$ \\ 
 & $2.00 \times$   & $85.00\%\pm2.94\%$ & $92.72\%\pm0.91\%$ & $42.82\%\pm26.72\%$ & $8.80\%\pm9.77\%$ & \hl{$94.52\%\pm0.80\%$} & $92.77\%\pm0.77\%$ \\
 \cmidrule{2-8}
 \multirow{4}{*}{\walker{}} 
 & $0.00 \times$   & \hl{$96.33\%\pm0.94\%$} & $95.33\%\pm1.89\%$ & $76.80\%\pm2.52\%$ & $75.67\%\pm1.04\%$ & $71.35\%\pm0.86\%$ & $83.03\%\pm0.63\%$\\
 & $0.01 \times$   & \hl{$64.67\%\pm5.25\%$} & $63.33\%\pm0.94\%$ & $13.75\%\pm4.64\%$ & $28.03\%\pm6.72\%$ & $26.83\%\pm1.47\%$ & $39.50\%\pm1.91\%$\\
 & $0.03 \times$   & $33.00\%\pm4.34\%$ & $33.60\%\pm4.96\%$ & $21.98\%\pm5.99\%$ & $33.84\%\pm2.63\%$ & $29.59\%\pm1.05\%$ & \hl{$39.02\%\pm1.40\%$} \\
 & $0.05 \times$    & $17.33\%\pm2.87\%$ & $21.33\%\pm0.94\%$ & \hl{$30.43\%\pm1.03\%$} & $21.90\%\pm2.15\%$ & $13.58\%\pm0.81\%$ & \hl{$29.92\%\pm3.74\%$} \\
\midrule
& & \multicolumn{5}{c}{\textbf{Data Efficiency}} \\
\midrule
 \multirow{5}{*}{\fetchpush{}} 
 & 20311  & $82.00\%\pm21.13\%$ & $89.40\%\pm2.06\%$ & $33.73\%\pm37.63\%$ & $91.64\%\pm9.08\%$ & \hl{$93.66\%\pm3.15\%$} & \hl{$95.78\%\pm0.80\%$} \\
 & 10000  & $80.20\%\pm14.70\%$ & $90.20\%\pm2.64\%$ & $24.18\%\pm31.75\%$ & $62.10\%\pm43.86\%$ & $55.79\%\pm45.62\%$ & \hl{$95.31\%\pm0.45\%$}\\
 & 5000   & $76.40\%\pm26.27\%$ & $86.60\%\pm2.15\%$ & $43.59\%\pm36.58\%$ & $77.60\%\pm38.91\%$ & $38.04\%\pm46.32\%$ & \hl{$95.70\%\pm0.75\%$}\\
 & 2000    & \hl{$80.20\%\pm14.70\%$} & \hl{$84.40\%\pm1.85\%$} & $33.28\%\pm24.07\%$ & $41.21\%\pm47.47\%$ & $46.61\%\pm37.37\%$ & \hl{$86.44\%\pm13.44\%$}\\
 \cmidrule{2-8}
 \multirow{5}{*}{\walker{}} 
 & 5 trajs & \hl{$5431.19\pm267.40$} & $4749.03\pm224.96$ & $3581.18\pm574.20$ & $2521.07\pm863.44$ & $4639.47\pm282.92$ & \hl{$5381.15\pm115.25$}\\
 & 3 trajs & $5061.72\pm73.57$ & $3476.26\pm313.01$ & $2837.76\pm1028.95$ & $3210.65\pm518.24$ & $4584.24\pm200.69$ & \hl{$5266.41\pm57.93$}\\
 & 2 trajs & \hl{$4957.94\pm658.54$} & $1872.29\pm325.88$ & $2323.08\pm886.06$ & $2067.75\pm409.50$ & $3250.23\pm1610.07$ & \hl{$5083.32\pm119.98$}\\
 & 1 traj  & $3055.27\pm1834.75$ & $1165.29\pm147.79$ & $960.65\pm79.89$ & $1017.37\pm47.21$ & $3057.35\pm1530.88$ & \hl{$4960.10\pm164.57$}\\
\bottomrule 
\end{tabular}}
\label{table:img_arch}
\end{table*}
